# Supplementary material for: NerVE: Neural Volumetric Edges for Parametric Curve Extraction from Point Cloud
Source: arXiv:2303.16465 source file (2023-03-29)
Supplement: Supplementary file 1 [file Supp_complex.tex]

\begin{figure*}[!t]
	\centering
	\includegraphics[width=1.\linewidth]{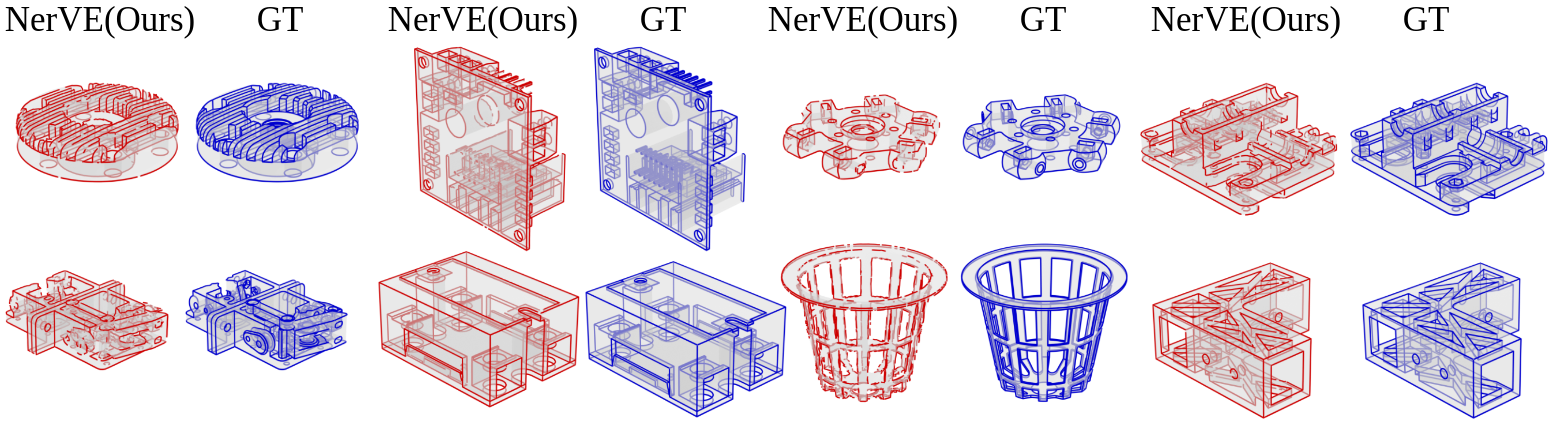}
	\caption{Results of predicted PWL curves using our method on some complicated cases.}
	\label{fig:complex_cases}
	\vspace{-5mm}
\end{figure*}
